# Supplementary material for: Improving the accuracy of neutrino energy reconstruction in charged-current quasielastic scattering off nuclear targets
Source: arXiv:1404.5687 ancillary file (2015-02-17)
Supplement: Supplementary file 1 [file CrossSections.pdf]

# Improving the accuracy of neutrino energy reconstruction in charged-current quasielastic scattering off nuclear targets. Supplemental Material

Artur M. Ankowski,[1,*] Omar Benhar,[2] and Makoto Sakuda[1]

[1] *Department of Physics, Okayama University, Okayama 700-8530, Japan*

[2] *INFN and Department of Physics, "Sapienza" Università di Roma, I-00185 Roma, Italy*

Figures 1–5 show comparisons between the results of our calculations and the $^{12}_{6}\mathrm{C}(e,e')$ data reported in Refs. [1–8], spanning a broad kinematical region.

In addition to those collected at low scattering angles and moderate momentum transfers, we include here the data sets obtained at kinematical setups in which reaction mechanisms other than quasielastic scattering are known to play an important role. Most notably, the contribution of meson exchange currents, of a transverse nature, strongly affects the measured cross sections at large scattering angle.

We believe that this work provides new insight on the kinematical range in which the proposed approach describes the electron-scattering data accurately, and gives an accurate estimate of the quasielastic contribution to the cross section even in the kinematical conditions in which other reaction mechanisms become significant.

[1] D. T. Baran *et al.*, Phys. Rev. Lett. **61**, 400 (1988).
[2] O. Benhar, D. Day, and I. Sick, arXiv:nucl-ex/0603032.
[3] D. B. Day *et al.*, Phys. Rev. C **48**, 1849 (1993).
[4] D. S. Baghdassarian *et al.*, YERPHI-1077(40)-88.
[5] P. Barreau *et al.*, Nucl. Phys. A **402**, 515 (1983).
[6] J. S. O'Connell *et al.*, Phys. Rev. C **35**, 1063 (1987).
[7] R. M. Sealock *et al.*, Phys. Rev. Lett. **62**, 1350 (1989).
[8] R.R. Whitney, I. Sick, J.R. Ficenec, R.D. Kephart, and W.P. Trower, Phys. Rev. C **9**, 2230 (1974).

* Present address: Center for Neutrino Physics, Virginia Tech, Blacksburg, Virginia 24061, USA; artank@vt.edu

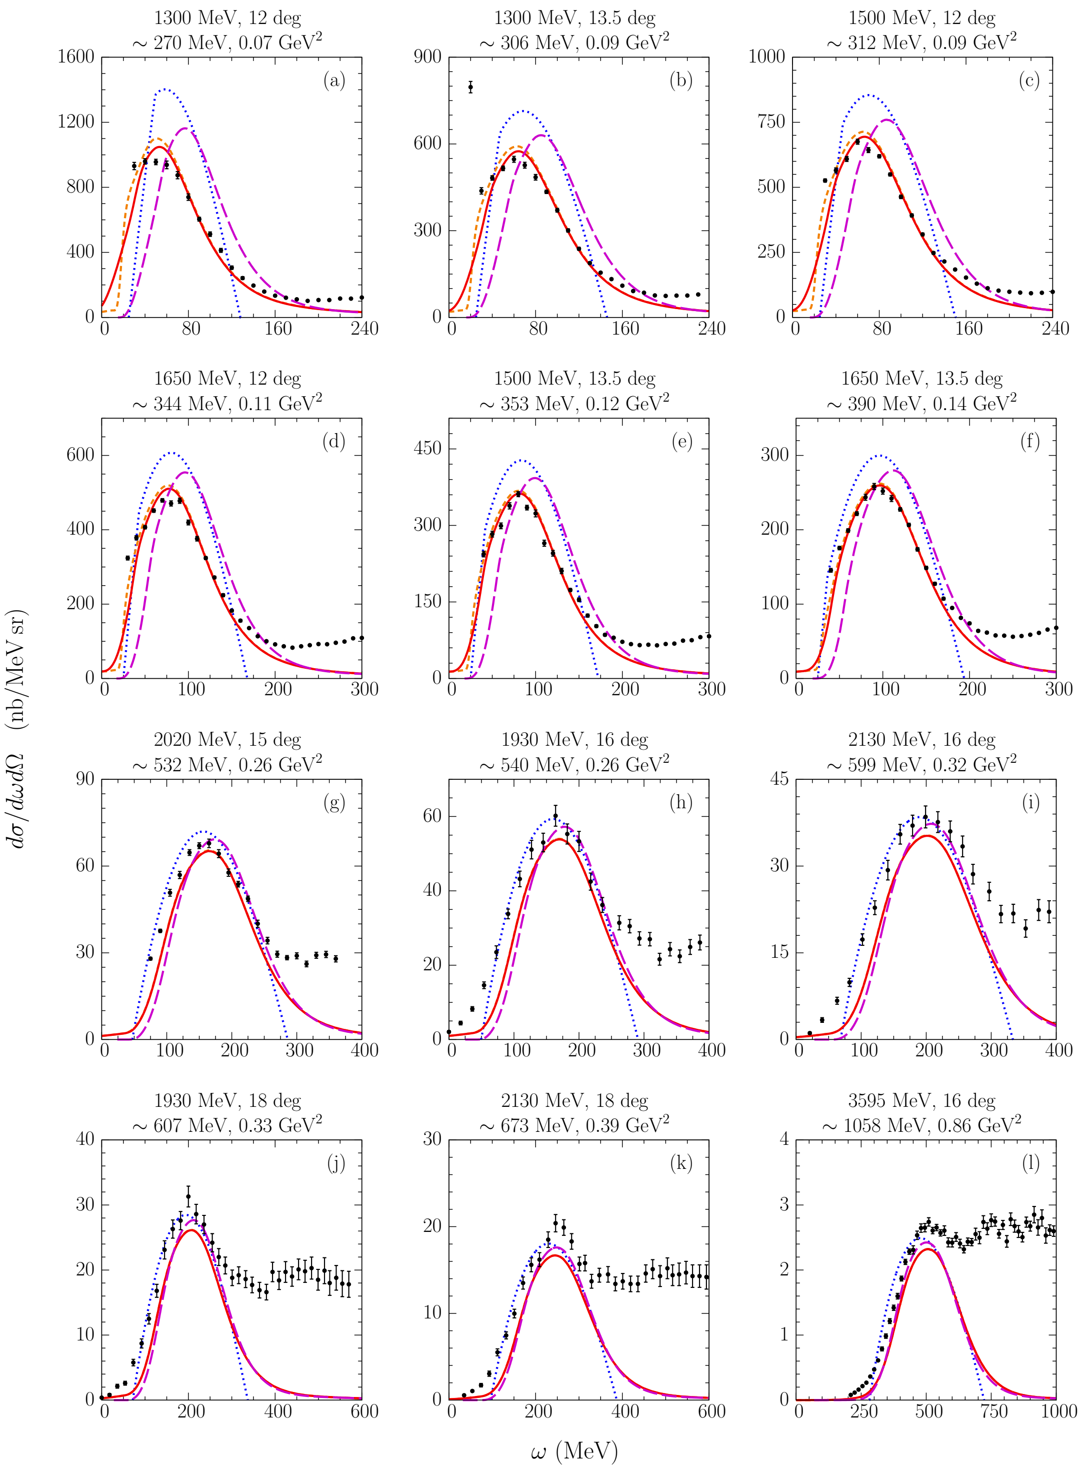


FIG. 1. Cross sections $d\sigma/d\omega d\Omega$ for electron scattering off carbon. Our results with Pauli blocking accounted for in the local-density (solid lines) and step-function (short-dashed lines) approximations are compared with the experimental data reported by Baran *et al.* [1, 2] [(a)–(f)], Day *et al.* [3] [(g) and (l)], and Baghdassarian *et al.* [4] [(h)–(k)]. The IA (long-dashed lines) and RFG calculations (dotted lines) are added for reference. The panels are labeled with beam energy, scattering angle, and values of $|\mathbf{q}|$ and $Q^2$ at the quasielastic peak.

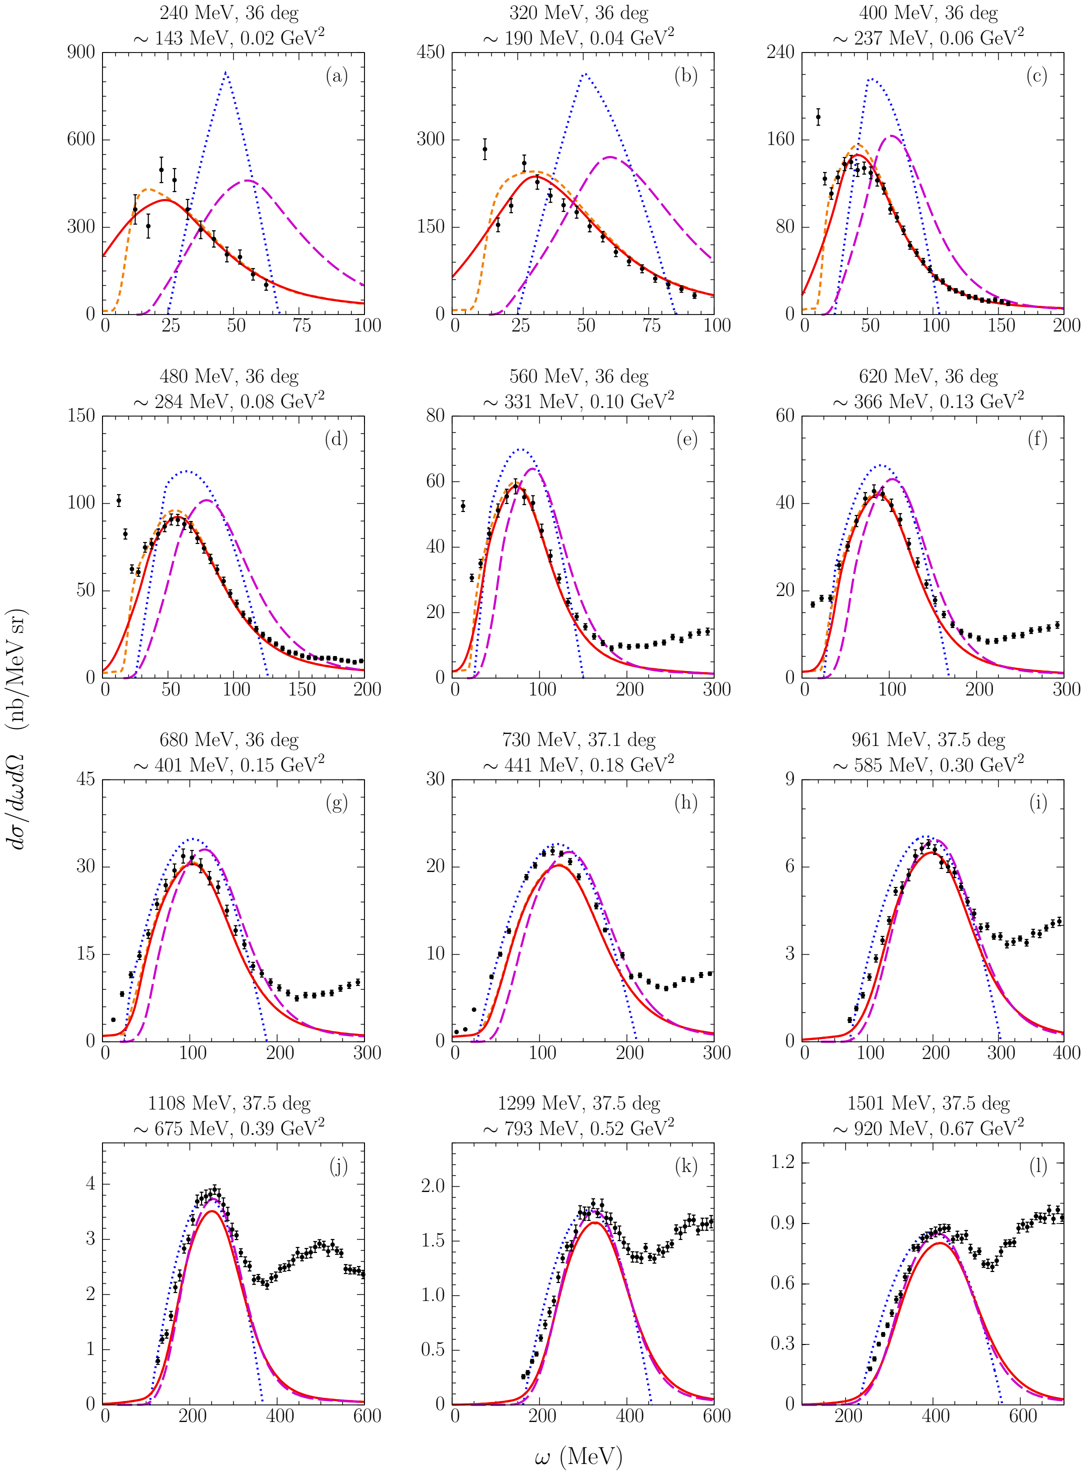


FIG. 2. Same as Fig. 1 but for the cross sections measured by Barreau *et al.* [5] [(a)–(g)], O'Connell *et al.* [6] [(h)], and Sealock *et al.* [7] [(i)–(l)].

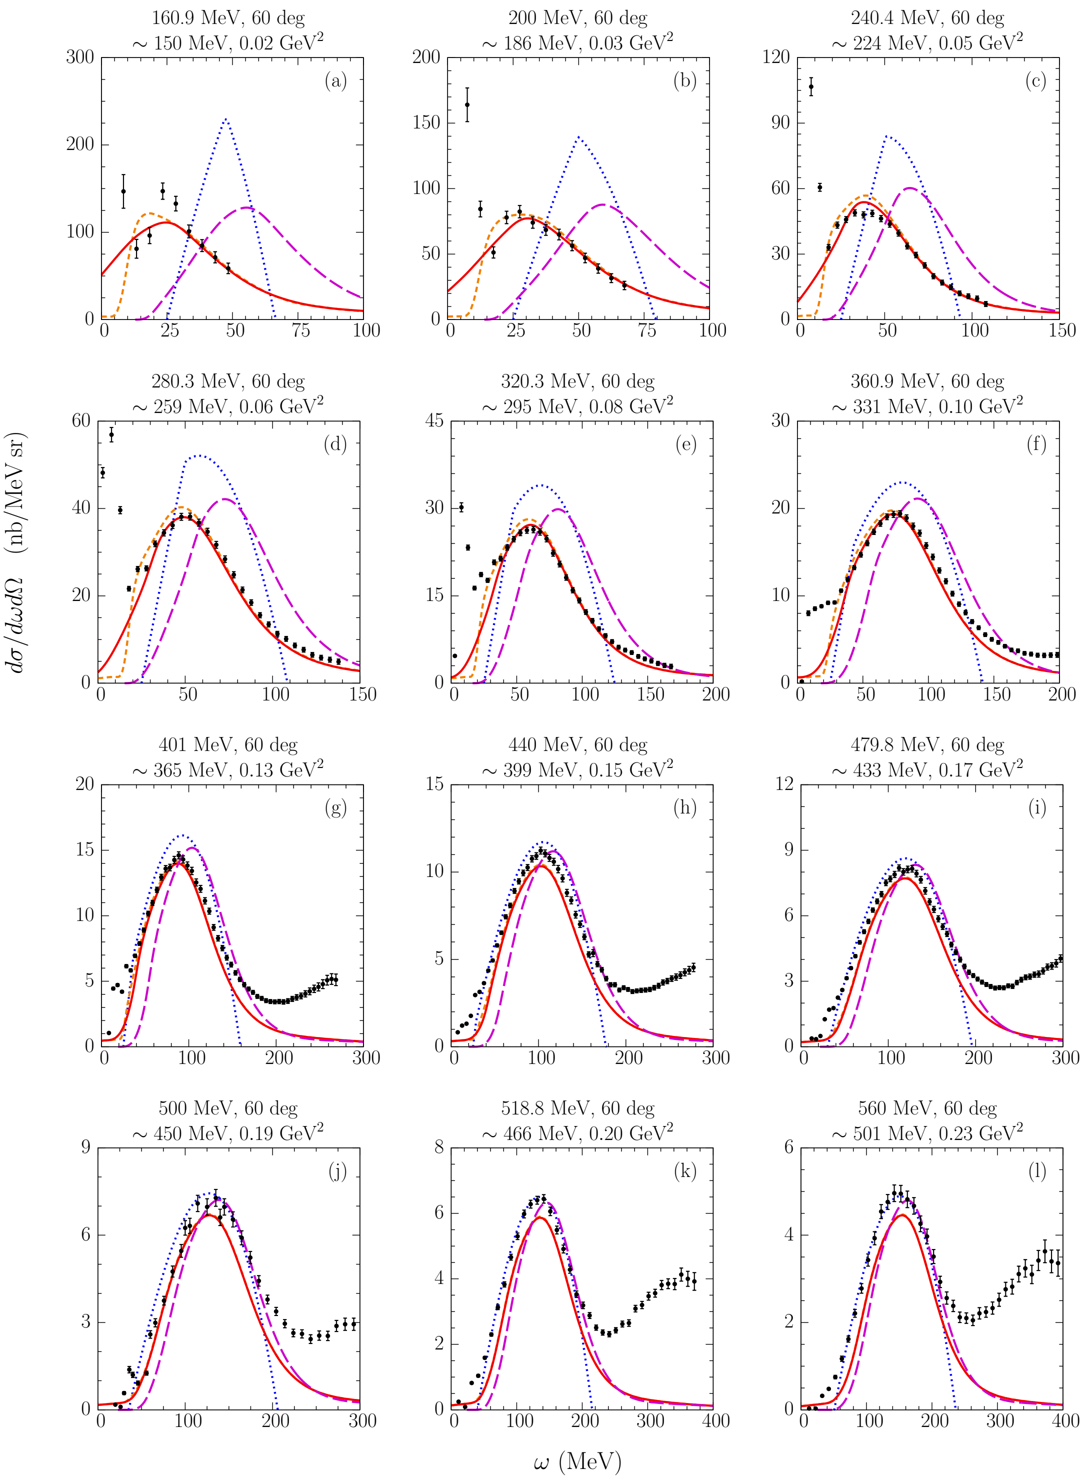


FIG. 3. Same as Fig. 1 but for the experimental data reported by Barreau *et al.* [5] [(a)–(i), (k) and (l)] and Whitney *et al.* [8] [(j)] for the scattering angle 60°.

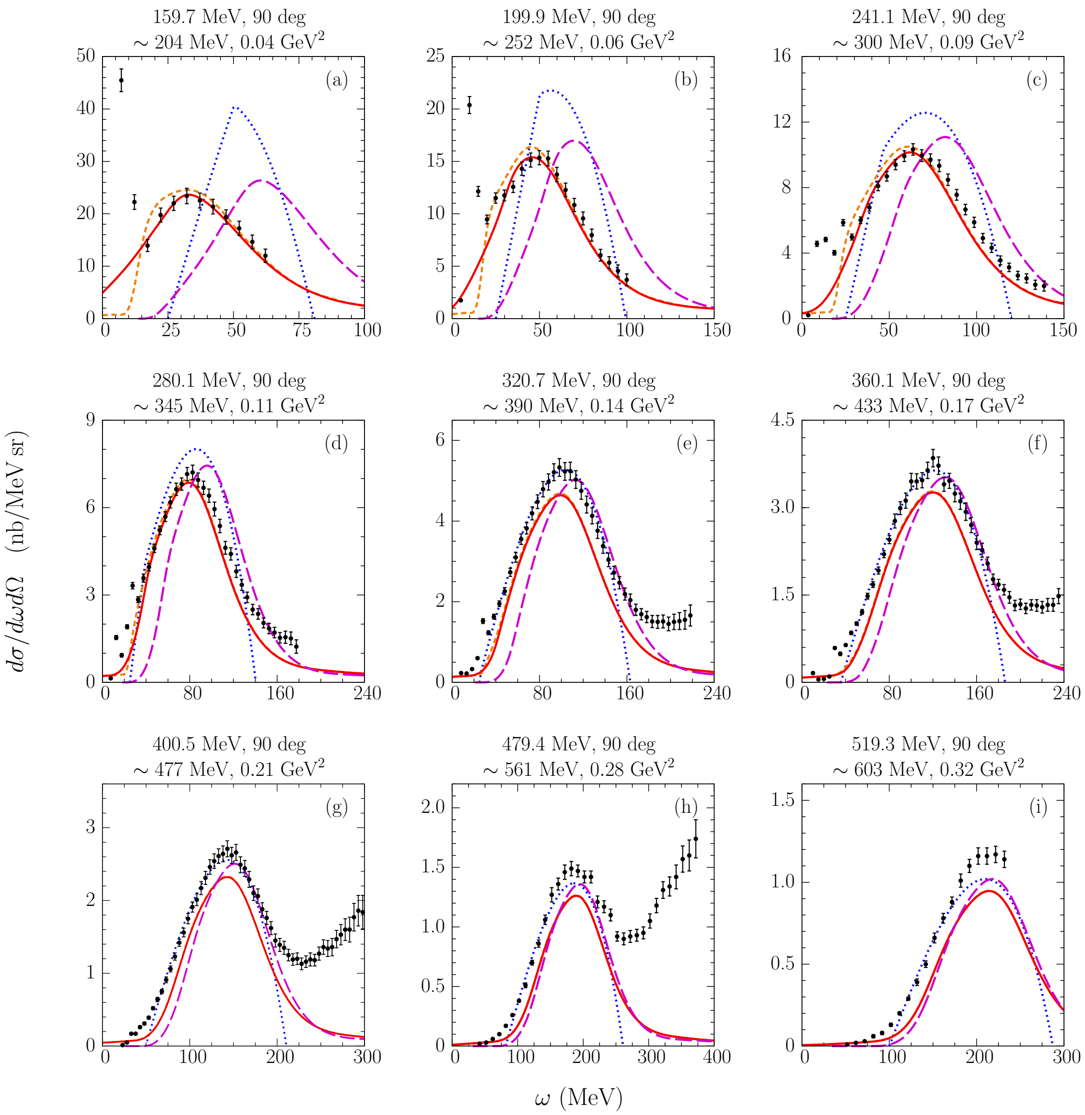


FIG. 4. Same as Fig. 1 but for the cross sections measured by Barreau *et al.* [5] at the scattering angle 90°.

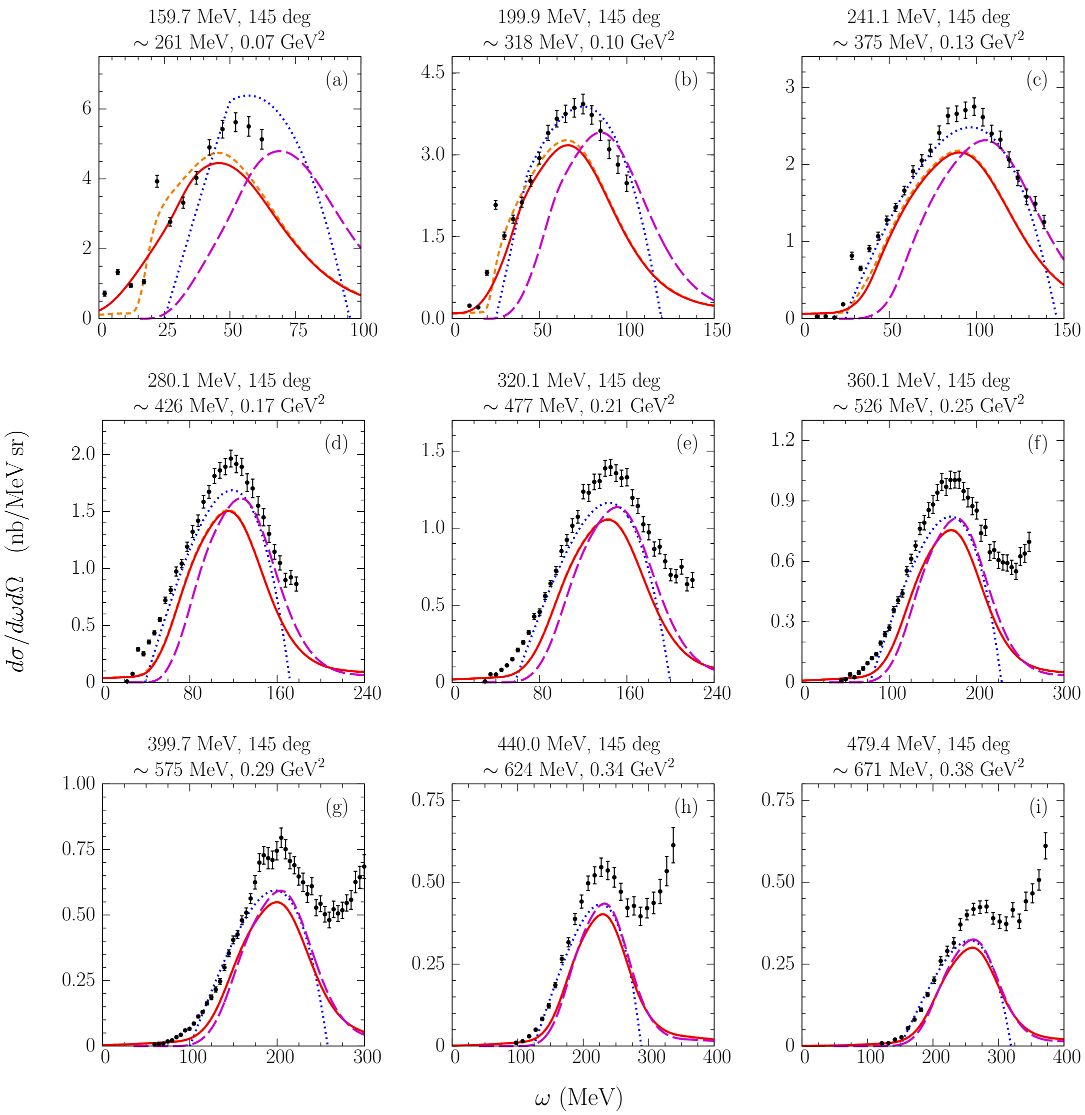


FIG. 5. Same as Fig. 1 but for the cross sections measured by Barreau *et al.* [5] at the scattering angle 145°.
